# Supplementary material for: Versatile AFM setup combined with micro-focused X-ray beam
Source: arXiv:1506.00561 source file (2015-06-02)
Supplement: Supplementary file 1 [file AFM_rev_sci_inst_supplements.pdf]

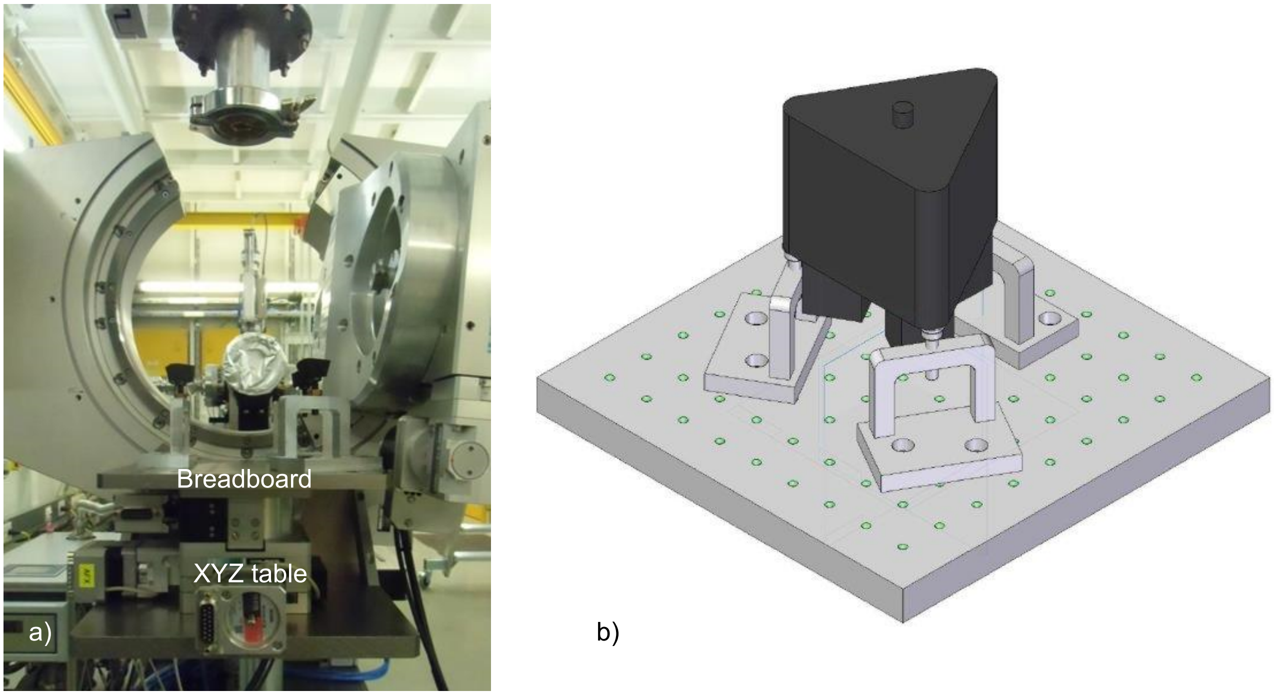


FIG. 1. (a) Adapter support unit mounted to the chi-circle of a Huber diffractometer. (b) Drawing of the breadboard with three pivots to support AFM body.

## SUPPLEMENTARY MATERIALS FOR: VERSATILE AFM SETUP COMBINED WITH MICRO-FOCUSED X-RAY BEAM

T. Slobodskyy, A.V. Zozulya, R. Tholapi, L. Liefeith, M. Fester, M. Sprung, W. Hansen.

## THIS PDF FILE DESCRIBES PERFORMANCE OF THE AFM SETUP MOUNTED AT THE P10 6-CIRCLE DIFFRACTOMETER.

In order to enable high resolution X-ray diffraction (HRXRD) experiments in combination with the AFM sample environment we have designed the adapter support equipped with X-, Y- and Z- motorized translation stages for sample alignment. The adapter support consists of L-shaped plate which can be mounted to the chi-circle of the Huber diffractometer as shown in Fig. 1 a). The base plate of the support unit is bearing the XYZ positioning tower based on Huber linear translations (100x100 mm size). On top of a XYZ tower the standard breadboard plate with M6 threaded holes is mounted. This plate is used as a base for the AFM support pivots as can be seen in Fig. 1 b).

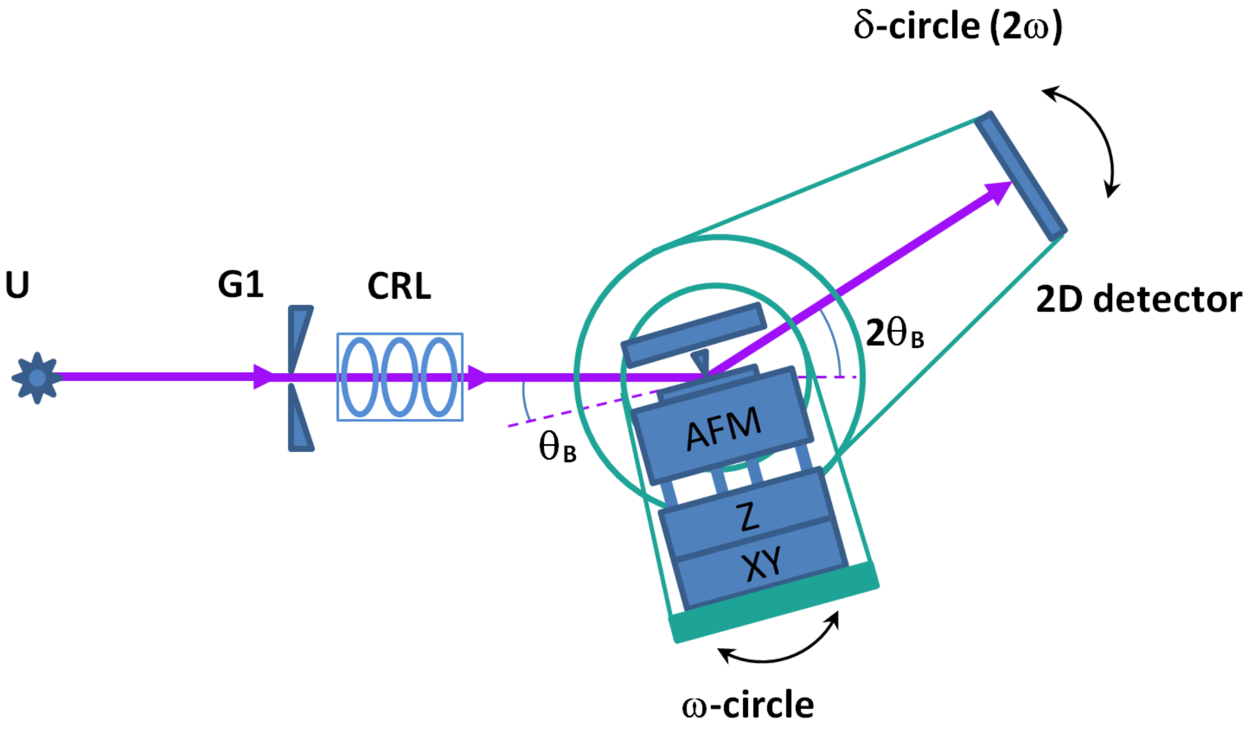


FIG. 2. Schematics of X-ray diffraction experiment using AFM at 6-circle diffractometer. U: undulator, G1: slits, CRL: compound refractive lenses.

The AFM body is placed on three supporting pivots and the assembled system is located on the six-circle diffractometer in EH1 of P10 beamline at 73.5 m from the undulator source. The first alignment step is to align the center of diffractometer to the X-ray beam. Then, using three translations of the XYZ tower the AFM, has to be translated to bring the sample to the center of the diffractometer. In this configuration the AFM can be straightforwardly aligned for X-ray diffraction experiments in vertical diffraction plane (Fig. 2). The conical openings in the AFM head are extending the range of accessible Bragg angles to the maximum exit angle of 20 degrees.

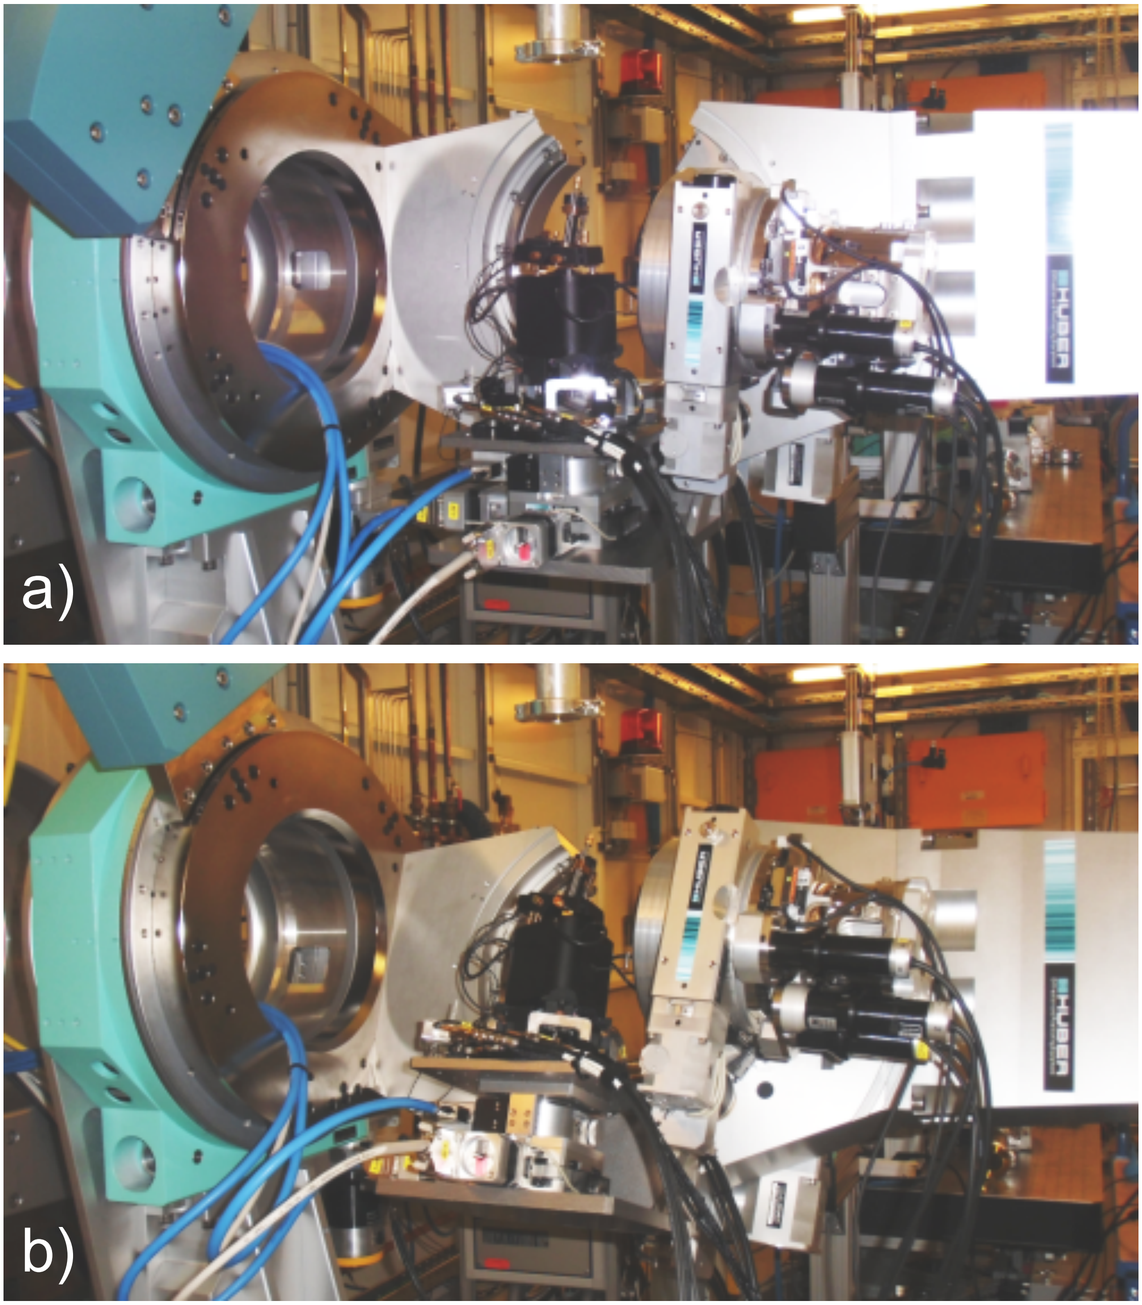


FIG. 3. AFM setup at 6-circle diffractometer positioned at (a) $\omega$=0 deg. and (b) $\omega$=20 deg.

Fig. 3 shows the AFM positioned at initial position of $\omega$=0 deg. and at inclined position of $\omega$=20 deg. The AFM is operational at these inclination angles.

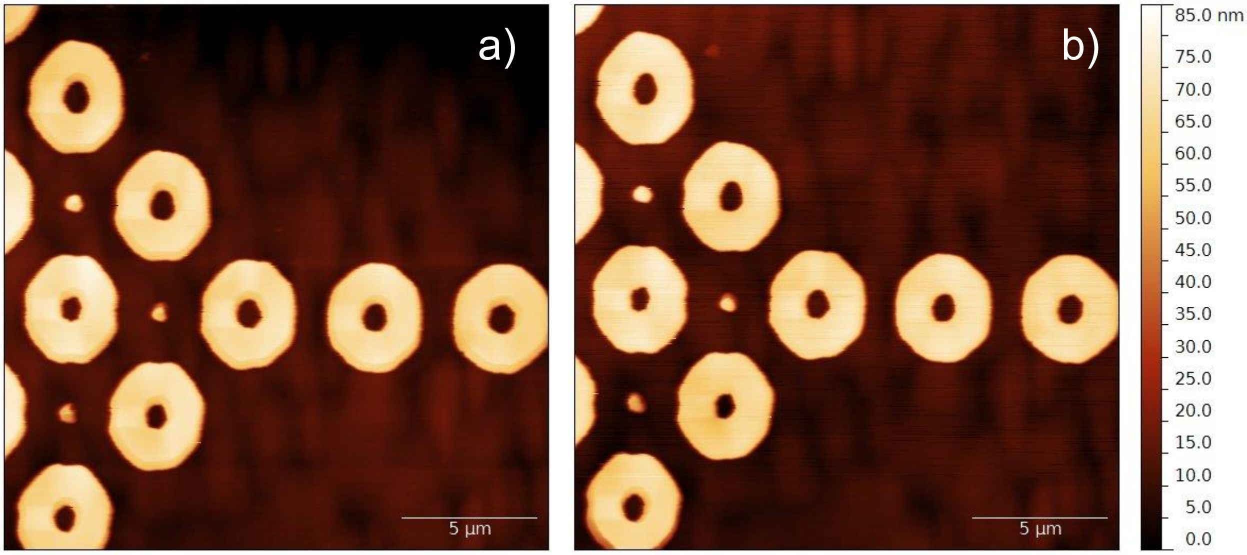


FIG. 4. AFM images of a bridge area of the MgO micro-ring structure acquired at (a) $\omega$=0 deg. and (b) $\omega$=20 deg.

In order to evaluate the performance of the AFM under the inclinations required during operation on the diffractometer we measured AFM images from the MgO micro-ring structures. AFM images measured at $\omega$=0 deg. and $\omega$=20 deg. are shown in Fig. 4. We observed only small deterioration of image quality at inclined position of the AFM setup, which indicates high stability of the discussed mounting design.
